# Supplementary material for: Augmented Physics: Creating Interactive and Embedded Physics Simulations from Static Textbook Diagrams
Source: arXiv:2405.18614 source file (2024-08-10)
Supplement: Supplementary file 1 [file 8-appendix.tex]

\section{Analyzed Websites}\label{appendix}

In the following tables (\autoref{tab:urls1} and \autoref{tab:urls2}), we list the interactive websites analyzed in Section 3. For each site, we provide the ID, name, and link, along with the identified design strategy, input method, and domain.

\begin{figure*}[h]
\centering
\includegraphics[width=0.8\textwidth]{draft-figures/Analysis.png}
\caption{Taxonomy analysis}
\label{fig:taxonomy-analysis}
\end{figure*}

\begin{table*}[b]

\small
\centering
\begin{tabulary}{\textwidth}{C L L L L L}
\textbf{ID} & \textbf{Name}                                                             & \textbf{Link}                                                                       & \textbf{\blue{Strategy}}                                 & \textbf{\green{Input}}                        & \textbf{\red{Domain}}            \\
\hline
1           & Visualize It - Trigonometric Functions                                    & \url{https://visualize-it.github.io/trig\\_functions/simulation.html}                      & Animated, Example, Reactive                      & Slider                                & Geometry                   \\
\hline
2           & Exponentiation - Explained Visually                                       & \url{https://setosa.io/ev/exponentiation/}                                                & Animated                                         & Slider                                & Applied Math, Arithmetic   \\
\hline
3           & Relating Area to Circumference                                            & \url{https://www.geogebra.org/m/w5rczf8n\#material/bq3gwxxn}                              & Animated, Exercise                                   & Direct, Text                          & Geometry                   \\
\hline
4           & Seeing circles, sines, and signals                                        & \url{https://jackschaedler.github.io/circles-sines-signals/index.html}                    & Animated                                         & Button, Direct, Slider                & Applied Math, Geometry     \\
\hline
5           & Systems of Linear Algebra                                                 & \url{https://textbooks.math.gatech.edu/ila/systems-of-eqns.html}                          & Example                                           & Direct, Slider                        & Algebra                    \\
\hline
6           & Let's remove Quaternions from every 3D Engine                             & \url{http://marctenbosch.com/quaternions/}                                                & Reactive                                          & Direct                                & Algebra, Geometry          \\
\hline
7           & Trigonometry for Games                                                    & \url{https://demoman.net/?a=trig-for-games}                                               & Animated, Example                                & Button, Direct                        & Geometry                   \\
\hline
8           & Back to the future of handwriting recognition                             & \url{https://jackschaedler.github.io/handwriting-recognition/}                            & Animated, Dynamic Calculation, Reactive          & Button, Direct, Slider                & Applied Math               \\
\hline
9           & Slower speed of light                                                     & \url{http://gamelab.mit.edu/games/a-slower-speed-of-light/}                               & Reactive                                          & Button, Direct                        & Algebra                    \\
\hline
10          & The Taxi Cab Problem                                                      & \url{http://galgreen.com/TaxiCabProblem/\#0}                                              & Example, Exercise                                     & Button, Slider                        & Probability                \\
\hline
11          & What Happens Next? COVID-19 Futures                                       & \url{https://ncase.me/covid-19/ }                                                         & Animated, Reactive                               & Button, Slider                        & Probability                \\
\hline
12          & Gears – Bartosz Ciechanowski                                              & \url{https://ciechanow.ski/gears/}                                                        & Animated                                         & Button, Slider                        & Applied Math               \\
\hline
13          & Seeing Theory Ch. 1: Basic Probability                                    & \url{https://seeing-theory.brown.edu/basic-probability/index.html}                        & Animated, Example, Reactive                      & Button, Direct                        & Probability                \\
\hline
14          & Going Critical — Melting Asphalt                                          & \url{https://meltingasphalt.com/interactive/going-critical/}                              & Animated, Contextual                                & Button, Slider                        & Probability                \\
\hline
15          & Graphs and Networks                                                       & \url{https://mathigon.org/course/graph-theory/introduction}                               & Contextual, Reactive                                 & Direct, Options, Text                 & Graph Theory               \\
\hline
16          & Quantum computing for the very curious                                    & \url{https://quantum.country/qcvc}                                                        & Exercise                                              & Button                                & Algebra                    \\
\hline
17          & An Interactive Introduction to Fourier Transforms                         & \url{https://www.jezzamon.com/fourier/index.html}                                         & Animated, Reactive                               & Button, Direct, Scroll, Slider        & Geometry                   \\
\hline
18          & The Wisdom and/or Madness of Crowds                                       & \url{https://ncase.me/crowds/}                                                            & Exercise, Reactive                                    & Direct                                & Graph Theory               \\
\hline

\end{tabulary}
    \caption{Documents analyzed in Study 1 (continued in \autoref{tab:urls2}). Each website is listed with the ID that identifies it in the paper, it's name, link, the design strategy, input method, and domain.}
    \label{tab:urls1}
\end{table*}

\begin{table*}[t]

\small
\centering
\begin{tabulary}{\textwidth}{C L L L L L}
\textbf{ID} & \textbf{Name}                                                             & \textbf{Link}                                                                       & \textbf{\blue{Strategy}}                                 & \textbf{\green{Input}}                        & \textbf{\red{Domain}}             \\
\hline
19          & Complexity Explorables | Horde of the Flies                               & \url{https://www.complexity-explorables.org/explorables/horde-of-the-flies/}              & Reactive                                          & Button, Slider                        & Probability                \\
\hline
20          & Visualizing the Impact of Feature Attribution Baselines                   & \url{https://distill.pub/2020/attribution-baselines/}                                     & Reactive                                          & Button, Hover, Slider                 & Applied Math               \\
\hline
21          & Exploring Bayesian Optimization                                           & \url{https://distill.pub/2020/bayesian-optimization/}                                     & Contextual, Reactive                                 & Slider                                & Probability                \\
\hline
22          & The Paths Perspective on Value Learning                                   & \url{https://distill.pub/2019/paths-perspective-on-value-learning/}                       & Animated                                         & Button, Slider                        & Applied Math               \\
\hline
23          & Computing Receptive Fields of CNN                                         & \url{https://distill.pub/2019/computing-receptive-fields/}                                & Reactive                                          & Hover, Slider                         & Applied Math               \\
\hline
24          & A Visual Exploration of Gaussian Processes                                & \url{https://distill.pub/2019/visual-exploration-gaussian-processes/}                     & Reactive                                          & Button, Slider                        & Applied Math, Probability  \\
\hline
25          & Understanding RL Vision                                                   & \url{https://distill.pub/2020/understanding-rl-vision/}                                   & Reactive                                          & Hover                                 & Applied Math               \\
\hline
26          & Seeing Theory Probability Distributions                                   & \url{https://seeing-theory.brown.edu/probability-distributions/index.html}                & Animated, Example, Reactive                      & Button, Direct, Options, Slider, Text & Probability                \\
\hline
27          & Firefly Synchronization                                                   & \url{https://visualize-it.github.io/firefly\\_synchronization/simulation.html}             & Animated, Example, Reactive                      & Button, Slider                        & Applied Math               \\
\hline
28          & Fourier Series                                                            & \url{https://visualize-it.github.io/fourier\\_series/simulation.html}                      & Dynamic Calculation,Example,Reactive              & Options, Slider                       & Applied Math               \\
\hline
29          & Markov Chains                                                             & \url{https://setosa.io/blog/2014/07/26/markov-chains/index.html}                          & Animated, Reactive                               & Slider                                & Applied Math, Graph Theory \\
\hline
30          & Pythagorean Theorem                                                       & \url{https://setosa.io/pythagorean/}                                                      & Reactive                                          & Direct                                & Geometry                   \\
\hline
31          & Sine and Cosine                                                           & \url{https://setosa.io/ev/sine-and-cosine/}                                               & Dynamic Calculation, Example, Reactive            & Direct                                & Calculus                   \\
\hline
32          & Vector Addition                                                           & \url{https://phet.colorado.edu/sims/html/vector-addition/latest/vector-addition\_en.html} & Dynamic Calculation, Example, Reactive            & Button, Direct, Slider, Text          & Algebra                    \\
\hline
33          & Polynomial Regression                                                     & \url{https://visualize-it.github.io/polynomial\_regression/simulation.html}               & Example, Reactive                                 & Direct, Slider                        & Applied Math, Calculus     \\
\hline
34          & Random Walks                                                              & \url{https://visualize-it.github.io/random\_walk/simulation.html}                         & Example                                           & Button                                & Probability                \\
\hline
35          & Porous Percolation                                                        & \url{https://visualize-it.github.io/porous\_percolation/simulation.html }                 & Animated, Example, Reactive                      & Button, Slider                        & Applied Math               \\
\hline
36          & Linear Transformations                                                    & \url{https://visualize-it.github.io/linear\_transformations/simulation.html}              & Animated, Example, Reactive                      & Button, Text                          & Algebra                    \\
\hline
37          & Mandelbrot Fractal                                                        & \url{https://visualize-it.github.io/mandelbrot\_fractal/simulation.html}                  & Animated                                         & Button                                & Applied Math               \\
\hline
38          & Bernoulli Percolation                                                     & \url{https://visualize-it.github.io/bernoulli\_percolation/simulation.html}               & Reactive                                          & Button, Slider                        & Applied Math               \\
\hline
39          & Hilbert Curve                                                             & \url{https://visualize-it.github.io/hilbert\_curve/simulation.html}                       & Animated                                         & Button                                & Applied Math               \\
\hline
40          & A Primer on Bézier Curves                                                 & \url{https://pomax.github.io/bezierinfo/}                                                 & Example, Reactive                                 & Direct, Slider                        & Applied Math, Geometry     \\
\hline
41          & A visual introduction to machine learning                                 & \url{http://www.r2d3.us/visual-intro-to-machine-learning-part-1/}                         & Animated                                         & Scroll                                & Applied Math, Probability  \\
\hline
42          & Conditional probability                                                   & \url{https://setosa.io/conditional/}                                                      & Animated, Dynamic Calculation, Example, Reactive & Slider                                & Probability                \\
\hline
43          & Pi ($\pi$)                                                                    & \url{https://setosa.io/ev/pi/}                                                            & Animated, Dynamic Calculation, Example, Reactive & Direct, Slider                        & Geometry                   \\
\hline

\end{tabulary}
    \caption{Documents analyzed in Study 1 (continued from \autoref{tab:urls1}). Each website is listed with the ID that identifies it in the paper, it's name, link, the design strategy, input method, and domain.}
    \label{tab:urls2}
\end{table*}
